# Supplementary material for: Computational Design of Alloy Nanostructures for Optical Sensing of Hydrogen
Source: arXiv:2204.06229 ancillary file (2022-06-30)
Supplement: Supplementary file 1 [file supporting-information.pdf]

# Computational Design of Alloy Nanostructures for Optical Sensing: The Limits of Tuning Hydrogen Sensitivity via Composition and Geometry

Pernilla Ekborg-Tanner, J. Magnus Rahm, Victor Rosendal,  
Tuomas P. Rossi, Tomasz J. Antosiewicz, and Paul Erhart

## Contents

|                                                                                                                    |           |
|--------------------------------------------------------------------------------------------------------------------|-----------|
| <b>Notes</b>                                                                                                       | <b>2</b>  |
| SN1. Lorentzian representation of dielectric functions . . . . .                                                   | 2         |
| SN2. Extinction spectra calculation with FDTD . . . . .                                                            | 2         |
| <b>Figures</b>                                                                                                     | <b>3</b>  |
| S1. Real part of dielectric function . . . . .                                                                     | 3         |
| S2. Imaginary part of dielectric function . . . . .                                                                | 3         |
| S3. Electronic density of states . . . . .                                                                         | 4         |
| S4. Extinction spectra for nanodisks with slightly different shape . . . . .                                       | 4         |
| S5. Extinction spectra for PdH <sub>x</sub> nanodisks with varying height and aspect ratio . . . . .               | 5         |
| S6. Absorption and scattering spectra . . . . .                                                                    | 6         |
| S7. Peak amplitude and position for PdH nanodisks . . . . .                                                        | 6         |
| S8. Extinction spectra and near fields at the resonances for PdH nanodisks . . . . .                               | 7         |
| S9. Hydrogen uptake in Pd–Au alloy as a function of Au concentration and H <sub>2</sub> pressure. . . . .          | 7         |
| S10. Peak shift sensitivity and disk diameter as a function of peak position . . . . .                             | 8         |
| S11. Sensitivity for Pd nanodisks of varying size and the corresponding RMSE of the linear fit . . . . .           | 8         |
| S12. Effect of artificial Gaussian broadening of extinction spectra . . . . .                                      | 9         |
| S13. Effect of size distribution on extinction spectra. . . . .                                                    | 9         |
| S14. Effect of order on extinction spectra and dielectric functions at Pd <sub>75</sub> Au <sub>25</sub> . . . . . | 10        |
| S15. Fitting of LR-TDDFT results to representation as sum of Lorentzians . . . . .                                 | 10        |
| <b>Supplementary References</b>                                                                                    | <b>11</b> |

## Notes

### Supplementary Note 1: Lorentzian representation of dielectric functions

To make the thus obtained DFs amenable to FDTD simulations with the MEEP software (1), they need to be represented as a sum of  $N$  Lorentzian functions,

$$\epsilon(\omega) = 1 + \sum_{j=1}^N \frac{x_j \omega_j^2}{\omega_j^2 - \omega^2 - i\omega\gamma_j} = 1 + \sum_{j=1}^N x_j L_j(\omega) \quad (1)$$

where  $x_j$ ,  $\omega_j$  and  $\gamma_j$  are parameters to be determined. As the computational cost has a direct dependence on the number of Lorentzians  $N$ , we want to keep  $N$  low. We have found the following strategy effective to determine  $N$ ,  $x_j$ ,  $\omega_j$  and  $\gamma_j$  such that the calculated DF are accurately represented (for a graphical illustration of the procedure, see Figure S15):

1. Create a matrix with elements  $A_{ij} = \text{Re } L_j(\omega_i)$  and  $A_{ij} = \text{Im } L_j(\omega_i)$  in the upper and lower parts, respectively. This matrix will have twice as many rows as there are frequencies  $\omega_i$  in the data obtained by LR-TDDFT in the frequency range to be fitted (one for the real part and one for the imaginary part; in our case we use 100 values of  $\omega_i$  in the photon energy range 0.7–10.7 eV for a total of 200 rows). Each column corresponds to a Lorentzian, and we use a 2D grid in the  $\omega_j$ – $\gamma_j$  plane with 200 values of  $\omega_j$  in the range (0–10.7 eV) and 200 values of  $\gamma_j$  logarithmically spaced in the range  $10^{-6}$  to  $10^2$  eV, for a total of 40,000 ( $\omega_j, \gamma_j$ ) pairs. The matrix  $A$  thus has dimensions  $200 \times 40,000$ .
2. With the thus obtained matrix we have an underdetermined system of equations  $A_{ij}x_j = \epsilon(\omega_i)$ , where  $\epsilon(\omega_i)$  are as-calculated values of the DF at discrete frequencies  $\omega_i$ . We solve this regression problem with the OMP (Orthogonal Matching Pursuit) algorithm as implemented in SCIKIT-LEARN (2) and wrapped in HIPHIVE (3). OMP allows us to control the sparseness of the solution, *i.e.*, the value of  $N$ . We test for values of  $N$  between 4 and 10 and choose the solution that has the lowest BIC (4) value.
3. Given the thus obtained solution with  $N$  oscillators, we fine-tune the  $3N$  parameters ( $x_j, \omega_j, \gamma_j$ ) by solving the non-linear system of equations (1) in a least-squares sense (with the left-hand side given by the as-calculated LR-TDDFT values), as implemented in SCIPY (5).

### Supplementary Note 2: Extinction spectra calculation with FDTD

During the FDTD simulations, Maxwell's equations are evolved in time until the intensity of the electric field at the disk center has decayed by a factor of at least  $10^{-6}$  from its previous maximum value. The power  $P_{\text{in}}(\omega)$  transmitted through a closed surface surrounding the nanodisk is calculated by integration of the Poynting vector. The absorption cross section  $\sigma_{\text{abs}}$  is then obtained by normalizing with the incoming intensity  $I(\omega)$ ,

$$\sigma_{\text{abs}}(\omega) = \frac{P_{\text{in}}(\omega)}{I(\omega)}. \quad (2)$$

The incoming intensity  $I(\omega)$  is calculated from a preceding simulation without the nanodisk and correspond to the transmitted power through a surface above the nanodisk normalized by area. Calculation of the scattering cross section  $\sigma_{\text{sca}}$  requires subtracting the fields from the preceding substrate-only simulation before calculating the transmitted power  $\tilde{P}_{\text{out}}(\omega)$  through a surface surrounding the nanodisk in the outward direction (as opposed to the inward direction for absorption),

$$\sigma_{\text{sca}}(\omega) = \frac{\tilde{P}_{\text{out}}(\omega)}{I(\omega)}. \quad (3)$$

Lastly, the extinction cross section  $\sigma_{\text{ext}}(\omega)$  can be calculated as the sum of absorption and scattering,

$$\sigma_{\text{ext}}(\omega) = \sigma_{\text{abs}}(\omega) + \sigma_{\text{sca}}(\omega). \quad (4)$$

## Figures

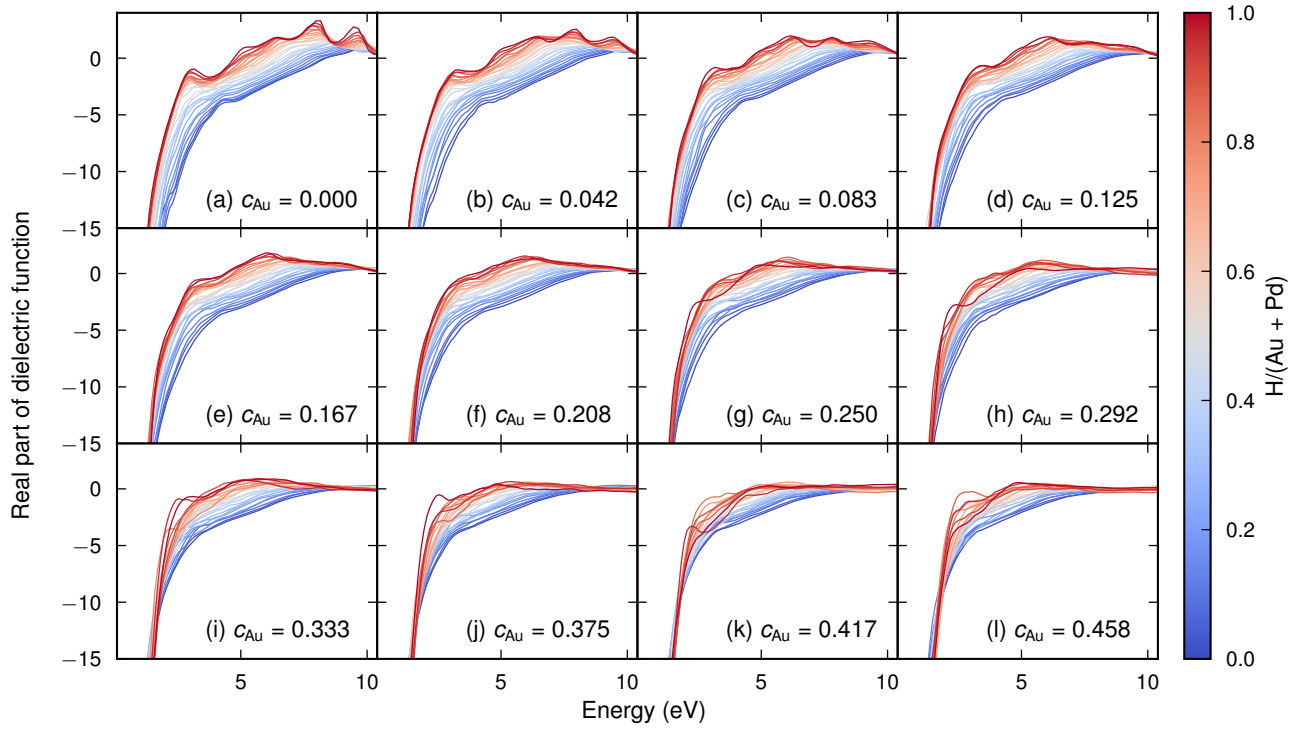

**Figure S1:** Real part of dielectric function for gold content ranging from 0 to 45.8% (a-l) and ranging from no hydrogen (blue) to full hydrogen loading (red).

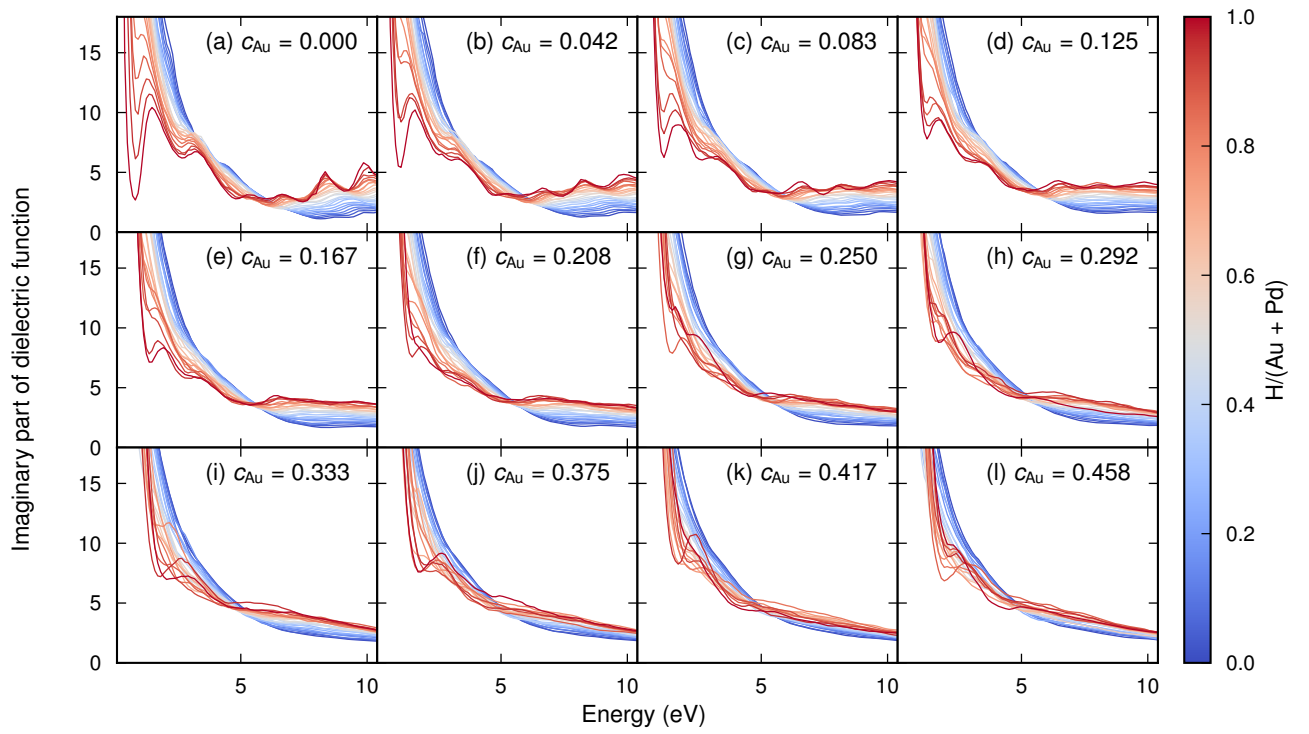

**Figure S2:** Imaginary part of dielectric function for gold content ranging from 0 to 45.8% (a-l) and ranging from no hydrogen (blue) to full hydrogen loading (red).

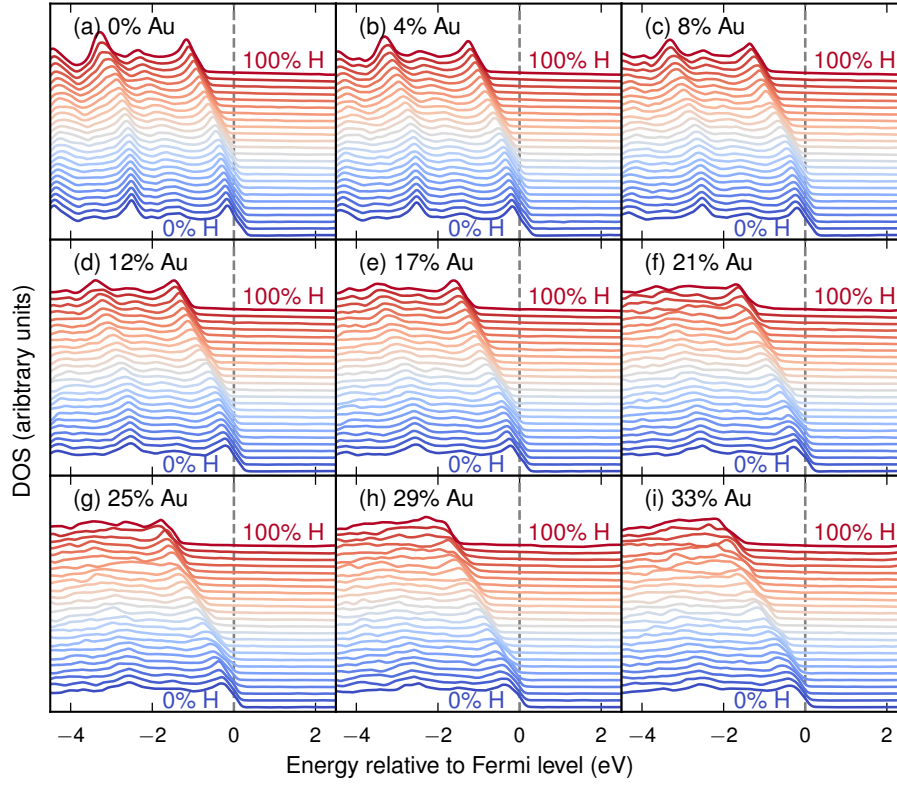

**Figure S3:** Electronic density of states at increasing Au content (a-i) in the range from no hydrogen (blue lines) to full hydrogen loading (red lines).

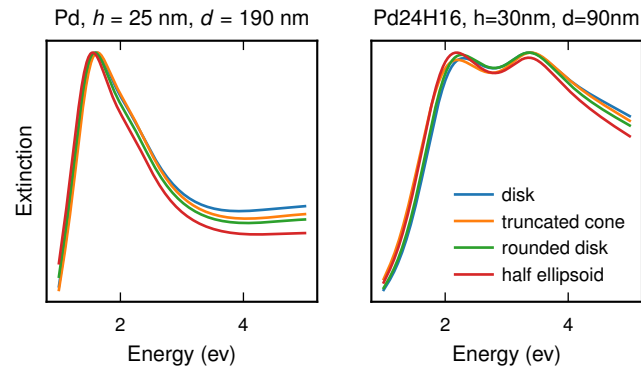

**Figure S4:** Extinction spectra for nanodisks with slightly different shape. The degree of rounding/tapering of the upper disk edge does not have a significant effect on the spectra.

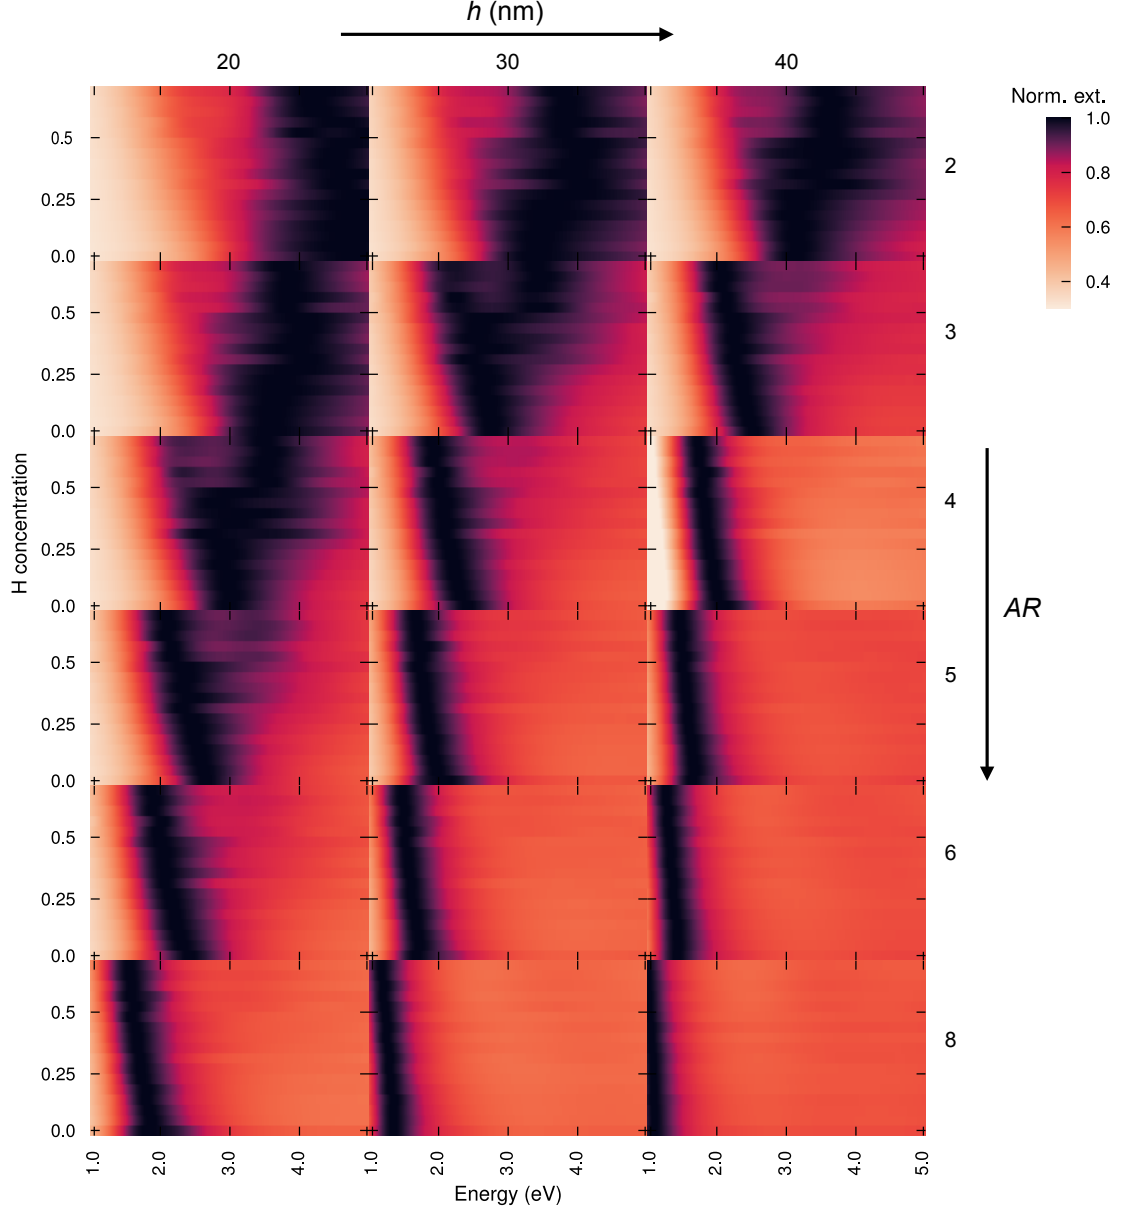

**Figure S5:** Extinction spectra for PdH<sub>x</sub> nanodisks with varying height  $h$  and AR. For the larger systems, we observe a single peak shifting to lower energies with increased H content, which is what is typically observed for LSPR H sensors. For smaller systems, e.g. for 30 nm  $\times$  3, a second peak appears with increased H content, shifting to higher energies. The peak splitting feature appear roughly over a diagonal in the figure. Above this imagined diagonal, we again observe a single peak but here it generally shifts to higher energies with increased H content, in contrast to the behavior for larger systems.

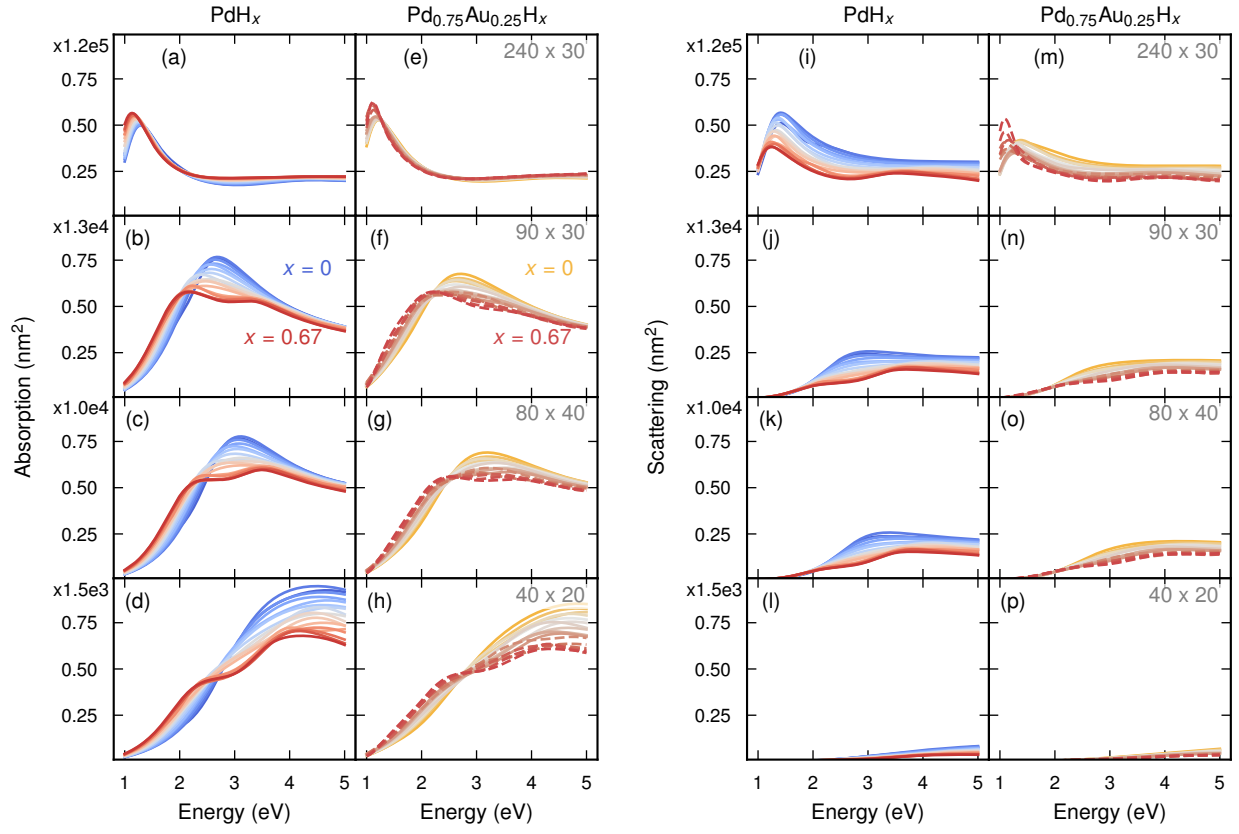

**Figure S6:** Absorption and scattering spectra for the same systems as in Figure 2.

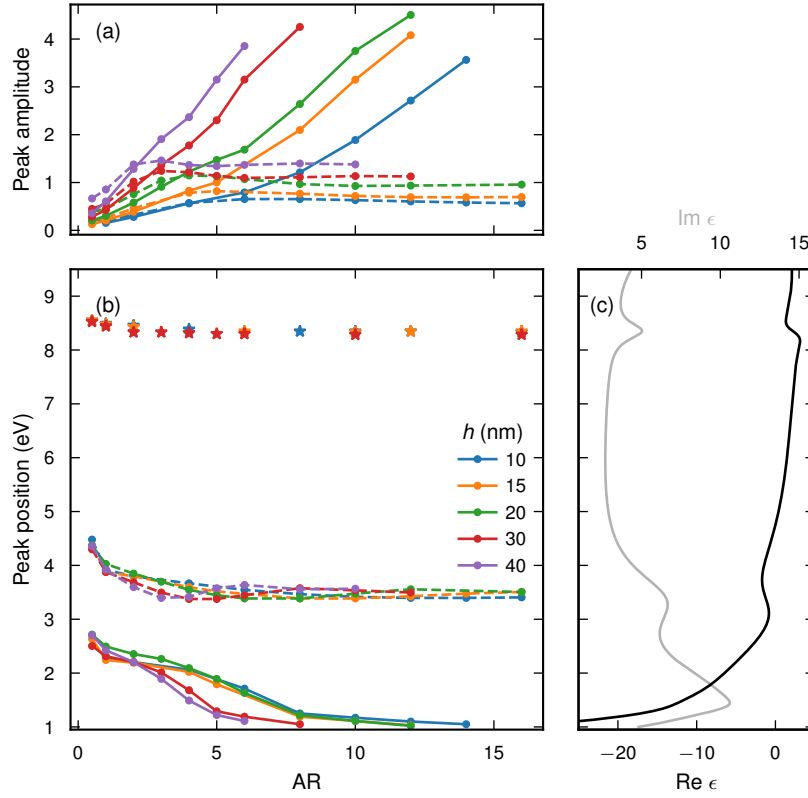

**Figure S7:** Peak amplitude (a) and position (b) for PdH nanodisks with varying height and AR and the corresponding dielectric function (c). With the extended energy interval, the connection between features in the DF and optical spectra is even more clear.

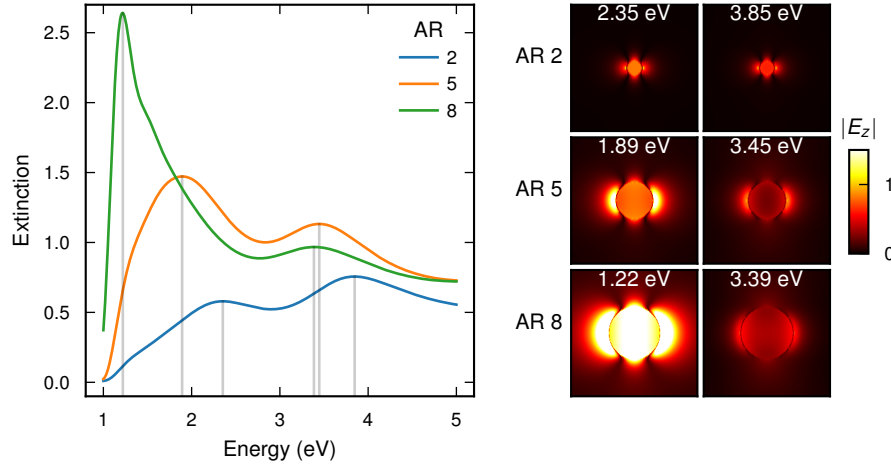

**Figure S8:** Extinction spectra and near fields at the resonances for PdH nanodisks with height 20 nm.

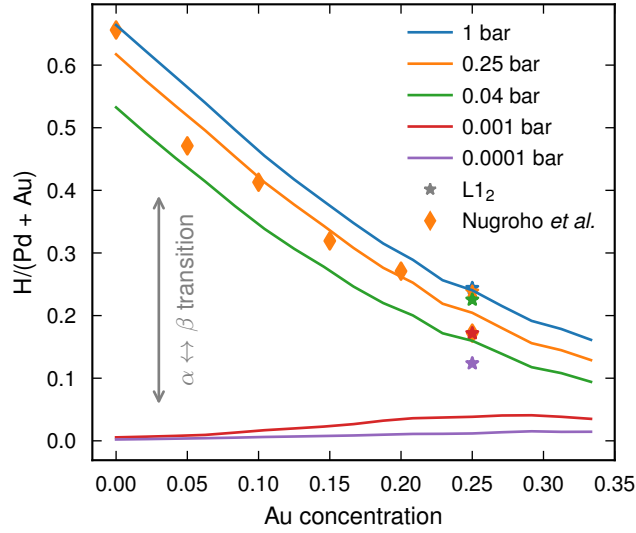

**Figure S9:** Hydrogen uptake in Pd–Au alloy as a function of Au concentration at pressures ranging from 0.1 mbar to 1 bar. Full lines show uptake when the Pd–Au sublattice is fully disordered, stars when the Pd–Au sublattice is ordered in the  $L1_2$  configuration. These data are based on the model and simulations developed in Ref. 6). Orange diamonds show hydrogen uptake experimentally determined in Ref. 7 using quartz crystal microbalance. The discontinuity in hydrogen uptake, which is particularly wide at low Au concentration, is a consequence of the phase transition between the dilute  $\alpha$  phase and the relatively dense  $\beta$  phase, which in pure Pd occurs just over 0.01 bar.

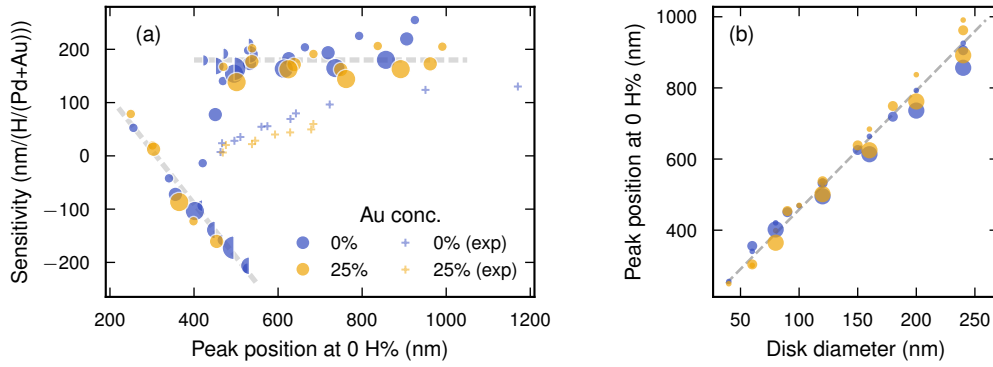

**Figure S10:** Peak shift sensitivity (a) and disk diameter (b) as a function of peak position at 0% H for varying Au concentration and disk heights 20, 30 and 40 nm (the marker size is proportional to height). The peak position follows a linear trend with respect to the disk diameter which is only slightly shifted with Au concentration or height.

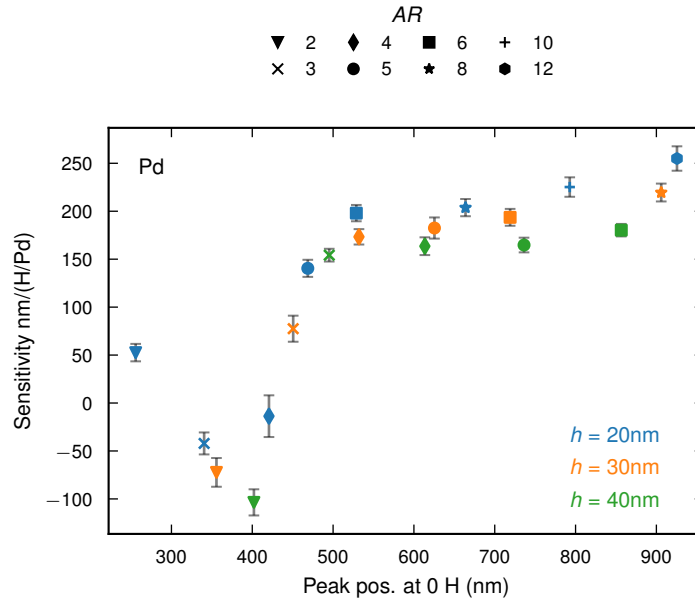

**Figure S11:** Sensitivity (based on peak shift) for Pd nanodisks of varying size and the corresponding RMSE of the linear fit. The RMSE is larger right before the sensitivity reaches the plateau, due to the large effect from peak splitting.



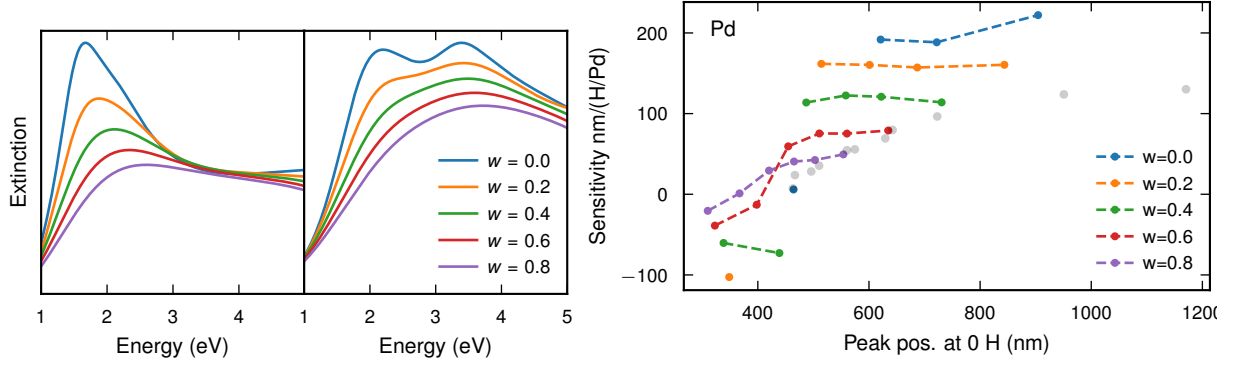

**Figure S12:** Effect of artificial Gaussian broadening of extinction spectra. The degree of broadening is determined by the width  $w$  of the Gaussian functions and  $w = 0$  corresponds to no broadening. By applying broadening, the sensitivity essentially changes from a step function to a roughly linearly trend, similar to what is observed experimentally.

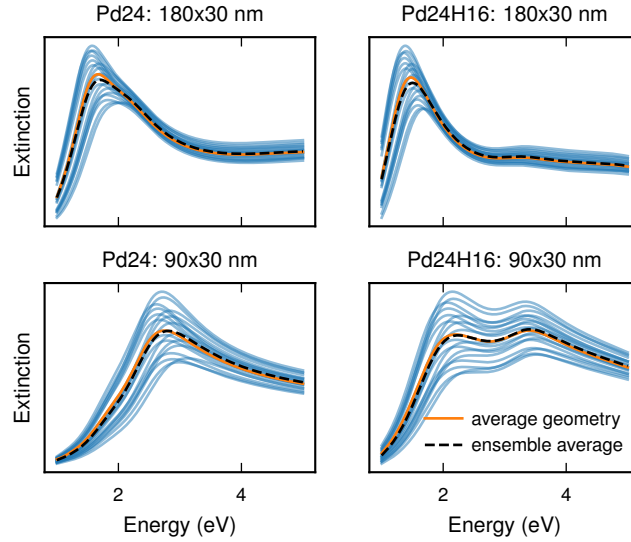

**Figure S13:** Effect of size distribution on extinction spectra. Two different geometries (specified as  $d \times h$ ) and compositions are considered, and the size distribution is introduced by varying the diameter uniformly in the interval  $d \pm 10\%$  while keeping the particle volume fixed (blue lines). The difference between the single particle spectra at the average geometry (orange line) and the ensemble average over the size distribution (black line) is very small, indicating that a uniform size distribution is not enough to introduce broadening of the extinction spectrum.

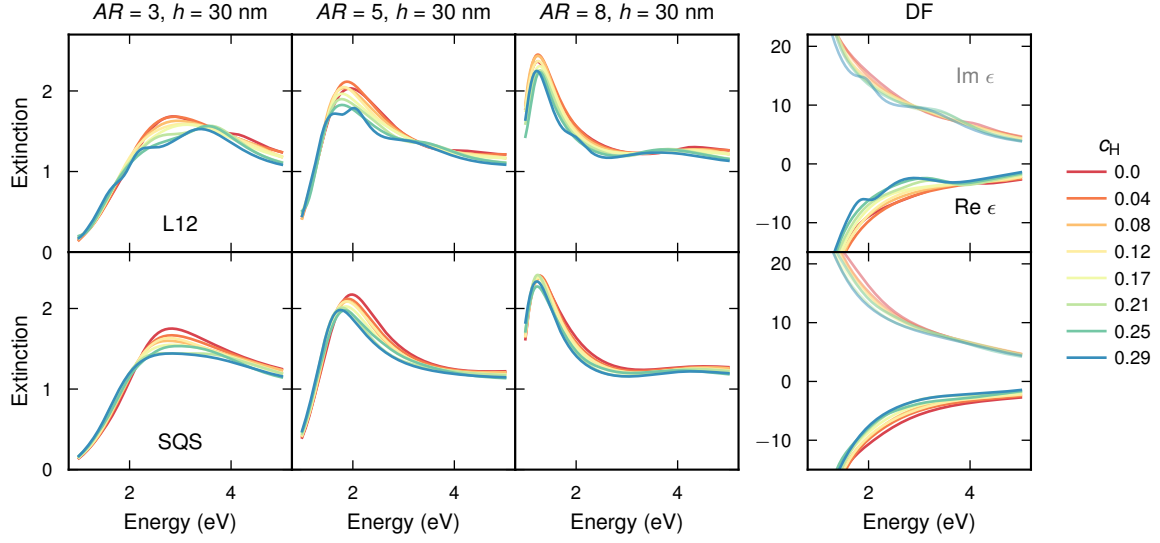

**Figure S14:** Extinction spectra and DFs for the ordered  $L1_2$  phase of  $\text{Pd}_{75}\text{Au}_{25}$  compared to disordered SQS of  $\text{Pd}_{75}\text{Au}_{25}$  at varying H content. The spectra share the same general features, although the  $L1_2$  structures have more fine structure. The fine structure would probably be averaged out in a real sample due to broadening, so we conclude that both cases should give similar measured optical response.

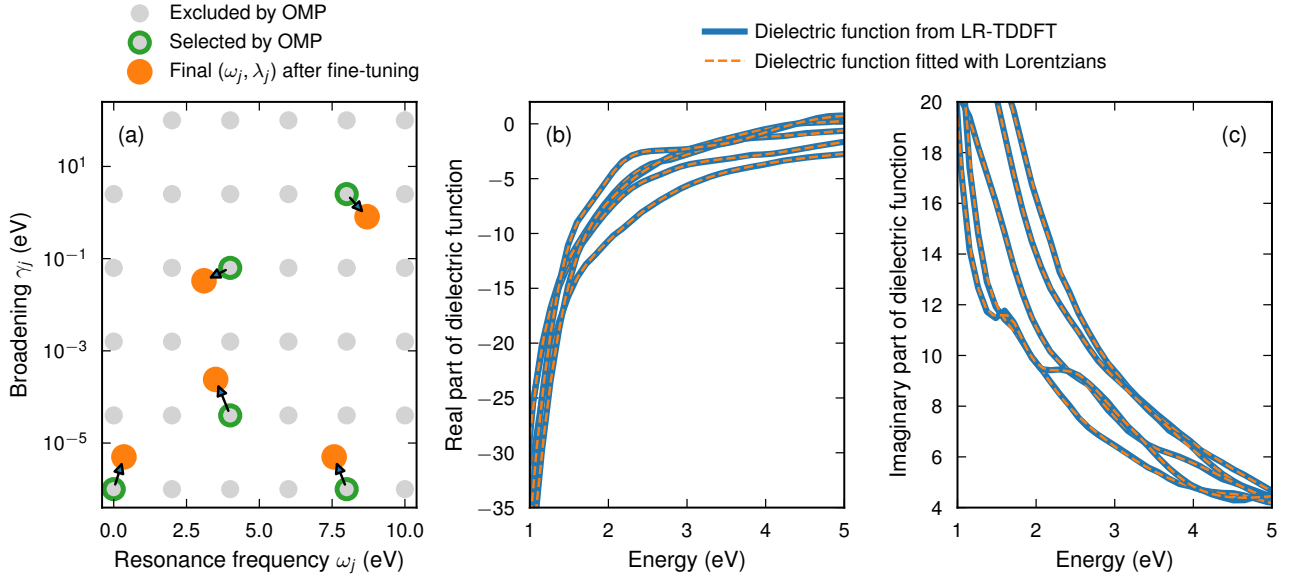

**Figure S15:** (a) Schematic overview of fitting of LR-TDDFT results to representation as sum of Lorentzians, as described in the Materials and Methods section of the main paper. A grid  $(\omega_j, \gamma_j)$  of Lorentzian frequencies and broadening parameters (grey circles) is created (in practice it is much denser than shown here), and Orthogonal Matching Pursuit (OMP) is used to select a small number (4–10) of Lorentzians that reproduce the LR-TDDFT data well (green circles). These Lorentzians are then fine-tuned by solving the non-linear problem (orange circles). (b–c) The resulting functions (orange, dashed lines) match the original data (blue lines) very well over the energy interval used for FDTD simulations, here exemplified by the dielectric functions of  $\text{Pd}_{0.75}\text{Au}_{0.25}$  with 0, 25, 50, 75, and 100% hydrogen.

## Supplementary References

- [1] A. F. Oskooi, D. Roundy, M. Ibanescu, P. Bermel, J. Joannopoulos, and S. G. Johnson, *Meep: A Flexible Free-Software Package for Electromagnetic Simulations by the FDTD Method*, Comput. Phys. Commun. **181**, 687 (2010). doi:<https://doi.org/10.1016/j.cpc.2009.11.008>.
- [2] F. Pedregosa, G. Varoquaux, A. Gramfort, V. Michel, B. Thirion, O. Grisel, M. Blondel, P. Prettenhofer, R. Weiss, V. Dubourg, J. Vanderplas, A. Passos, D. Cournapeau, M. Brucher, M. Perrot, and E. Duchesnay, *Scikit-learn: Machine Learning in Python*, J. Mach. Learn. Res. **12**, 2825 (2011).
- [3] F. Eriksson, E. Fransson, and P. Erhart, *The Hiphive Package for the Extraction of High-Order Force Constants by Machine Learning*, Adv. Theo. Simul. **2**, 1800184 (2019). doi:[10.1002/adts.201800184](https://doi.org/10.1002/adts.201800184).
- [4] G. Schwarz, *Estimating the Dimension of a Model*, Ann. Statist. **6**, 461 (1978).
- [5] P. Virtanen, R. Gommers, T. E. Oliphant, M. Haberland, T. Reddy, D. Cournapeau, E. Burovski, P. Peterson, W. Weckesser, J. Bright, S. J. van der Walt, M. Brett, J. Wilson, K. J. Millman, N. Mayorov, A. R. J. Nelson, E. Jones, R. Kern, E. Larson, C. J. Carey, Í. Polat, Y. Feng, E. W. Moore, J. VanderPlas, D. Laxalde, J. Perktold, R. Cimrman, I. Henriksen, E. A. Quintero, C. R. Harris, A. M. Archibald, A. H. Ribeiro, F. Pedregosa, P. van Mulbregt, and SciPy 1.0 Contributors, *SciPy 1.0: Fundamental Algorithms for Scientific Computing in Python*, Nat. Methods **17**, 261 (2020). doi:[10.1038/s41592-019-0686-2](https://doi.org/10.1038/s41592-019-0686-2).
- [6] J. M. Rahm, J. Löfgren, E. Fransson, and P. Erhart, *A Tale of Two Phase Diagrams: Interplay of Ordering and Hydrogen Uptake in Pd–Au–H*, Acta Mater. **211**, 116893 (2021). doi:[10.1016/j.actamat.2021.116893](https://doi.org/10.1016/j.actamat.2021.116893).
- [7] F. A. A. Nugroho, I. Darmadi, V. P. Zhdanov, and C. Langhammer, *Universal Scaling and Design Rules of Hydrogen-Induced Optical Properties in Pd and Pd-Alloy Nanoparticles*, ACS Nano **12**, 9903 (2018). doi:[10.1021/acsnano.8b02835](https://doi.org/10.1021/acsnano.8b02835).
